# Supplementary material for: SoftShadow: Leveraging Soft Masks for Penumbra-Aware Shadow Removal
Source: arXiv:2409.07041 source file (2025-03-12)
Supplement: Supplementary file 1 [file X_suppl.tex]

\clearpage
\maketitlesupplementary

In this supplementary material, we include more implementation details on the proposed SoftShadow model (Section~\ref{implementation_details}), mask sensitivity test for SOTA methods (Section~\ref{sensitive test}), soft and hard shadow image examples on well-used datasets (Section~\ref{shadow example}), and more visual results of our SoftShadow on the SRD dataset (Section~\ref{visual results}). 

\section{Implementation details}
\label{implementation_details}
Due to the computational cost, there are three training stages. We first finetune SAM~\cite{kirillov2023segment} for 100 epochs with a fixed learning rate of 1e-4, and we set $\lambda_1=0.1$. Next, we use the soft masks predicted by the tuned SAM to finetune ShadowDiffusion~\cite{guo2023shadowdiffusion} for another 500 epochs because the diffusion model~\cite{ho2020denoising} requires more epochs to reach convergence. The learning rate is set to 1e-5. Finally, we train SAM and ShadowDiffusion jointly for 500 epochs, with $\lambda_1=0.1$, $\lambda_2=1$, and the learning rate is set to 1e-5. We use Adam~\cite{kingma2014adam} optimizer for all training stages. We experiment with the hyperparameters $\lambda_1$ and $\lambda_2$  within the range of 0.01 to 1. To find the optimal learning rate, we tried setting the learning rate to values between 1e-4 and 1e-6. Empirically, the models work best when the learning rate is 1e-5 while a smaller or larger learning rate could lead to underfitting or model collapse.

For the input size, SAM requires a 1024$\times$1024 RGB image as the input, so we resize our image from 640$\times$840 to 1024$\times$1024. The output mask size from SAM is 256$\times$256. In ShadowDiffusion, we train with image and mask size set to 256$\times$256. We train the model with 2 GPUs and the total batchsize is set to 16 for all three stages. When finetuning SAM, we accumulate the gradient for 4 steps and the total batchsize for each step is 4. Compared to SAM Adapter~\cite{chen2023sam}, our implementation requires much less video memory to train the entire model, making our method more efficient and hardware-friendly. SAM Adapter requires around 60GB of video memory when batchsize is 4, which can only be met by GPUs such as A100 80GB, and H100. In contrast, our method requires 37GB of video memory and can be run on GPUs such as A100 40GB. In practice, we train the model on two A100 40GB and it is totally feasible to train the model on RTX series GPUs.
\section{Mask Sensitivity Evaluation}
\label{sensitive test}
% \begin{table}[t]
% \centering
% %\setlength{\tabcolsep}{1.5mm}
% \small  % This sets the font to approximately 9 point
% \begin{tabular}{c|ccc}
% \hline\hline
% Methods& ShadowDiffusion & HomoFormer &Ours\\
% \hline
% GT mask & \textbf{35.67} & \textbf{35.35} & \multirow{5}{*}{35.00} \\
% Otsu mask& \textbf{35.62} &33.47 & \\
% BDRAR mask& 33.41& 32.96&  \\
% FDRNet mask& 34.08& 32.41 & \\
% SAM Adapter & \textbf{35.32} & 33.34 &  \\
% \hline
% Mean & 34.82& 33.51 &N/A\\
% Std Dev & 0.831& 0.906&N/A\\
% \hline\hline
% \end{tabular}
% \caption{The stability test on ISTD+ dataset. The values in the table are PSNR results. The results that are higher than ours are \textbf{boldfaced}. }
% \label{ISTD+}
% \end{table}

\begin{table}[t]
\centering
\small  % This sets the font to approximately 9 point
\begin{tabular}{c|c|c|c}
\hline\hline
Input Masks& ShadowDiffusion & HomoFormer &Ours\\
\hline
Otsu mask& 35.02 & 26.26& \multirow{4}{*}{\textbf{35.57}}\\
\cline{1-3}
DHAN mask & 34.73 & \underline{35.37} &  \\
FDRNet mask & 33.39&21.01 &\\
Pretrained SAM & 31.30 & 18.22 &  \\
\hline
Mean & 33.61& 25.48&N/A\\
Std Dev & 1.469& 6.519&N/A\\
\hline\hline
\end{tabular}
\caption{The stability test on SRD dataset. The values in the table are PSNR results. The best result is~\textbf{boldfaced}. The second best result is~\underline{underlined}, respectively.}
\label{SRD}
\end{table}

In Section~\ref{mask_sensitivity}, we explore the mask sensitivity task within the ISTD+ dataset. The mask comparison is shown in Figure~\ref{istd_mask}. 
Since the ISTD+ dataset includes ground truth masks, it is not feasible for our methods to outperform the latest state-of-the-art (SOTA) approaches that rely on these ground truth masks during inference. However, we achieve comparable results without utilizing external masks, demonstrating the robustness of our approach.

We also evaluate the sensitivity on the SRD dataset, which does not have include ground truth masks provided. Most methods rely on the DHAN mask during inference. To provide a comprehensive evaluation, we test masks detected by DHAN~\cite{cun2020towards}, Otsu~\cite{hu2019mask}, FDRNet~\cite{zhu2021mitigating} and the pretrained SAM~\cite{kirillov2023segment}. Note that the detector FDRNet is trained on the ISTD~\cite{wang2018stacked} datasets. We do not distinguish between the ISTD and ISTD+ datasets here because the difference in illumination does not affect the position of the shadows.  We use the same pretrain model trained on the ISTD dataset to generate the mask on the SRD dataset. So the mask quality decreases because of the domain gap. The results are shown in Table~\ref{SRD}, the values shown are PSNR. Since our method does not require mask inputs, our results remain consistent across all tests. Our method outperforms all others. Although HomoFormer achieves comparable results with DHAN masks~\cite{cun2020towards}, it struggles to remove shadows with other mask inputs. The PSNR results for HomoFormer drop considerably when using alternative masks, despite showing strong performance with DHAN masks. This discrepancy might be due to HomoFormer being slightly overfitted to the style of DHAN masks, which include many small regions in the shadow masks, as illustrated in Figure~\ref{srd_mask}.

The mask we used is shown in the Figure~\ref{istd_mask}. From the mask, because Otsu use shadow-free image information, its mask is better than other methods. Compared with other mask detecters, we extract the more accurate mask. 

In sum, the sensitivity test suggests that previous methods, e.g., HomoFormer, can be sensitive to the quality of the input mask. This can be a problem for end users as variations in the input mask could lead to drastically different results while our method does not require external masks, making the usage more straightforward and robust against user error.

\begin{figure*}[t]
    \centering
    \includegraphics[width=1\textwidth]{figures/supp_srd_mask.png}
    \caption{Illustrate the soft shadow image examples in the SRD dataset. The red boxes highlight the boundaries and regions of soft shadows, showcasing their blurry boundaries and gradual transitions in the penumbra area.}
    \label{srd_mask}
\end{figure*}

\section{Shadow Image Examples}
\label{shadow example}
In this section, we present examples of soft shadows from the SRD~\cite{qu2017deshadownet} and LRSS~\cite{gryka2015learning} datasets, as well as hard shadow examples from the ISTD+~\ref{srd_sample}, the SRD dataset contains numerous soft shadow scenarios, the image varies in color, texture, and illumination. These soft shadows can be categorized into two types: blurry boundaries of large object shadows and small soft shadow regions. Shown in the first row and second row of Figure~\ref{srd_sample}, respectively. In Figure~\ref{lrss_sample}, the boundary of shadows is more blurry than it is in the SRD dataset. The LRSS dataset has limited diversity in background colors and textures. Figure~\ref{istd+_sample} shows that the shadows in the ISTD+ dataset are more hard shadows, which have sharp boundaries compared with shadow images on SRD or LRSS datasets. The ISTD+ dataset also offers less diversity in image scenarios compared to the SRD dataset.

\section{More Visual Results}
\label{visual results}
In this section, we present more soft shadow examples on SRD datasets. Figure~\ref{SUPP} shows visual comparisons with other SOTA methods that require external masks on the SRD dataset, the masks they used are DHAN masks~\cite{cun2020towards}. We can observe that our SoftShadow has better removal results on the soft boundaries of large object shadows and in small shadow regions. We show more visual comparison in Figure~\ref{SUPP_2} with other end-to-end methods that do not need shadow mask inputs. We can observe that our Softshadow removes shadow more precisely in shadow areas.

% \clearpage

\begin{figure*}[h]
    \centering
    \includegraphics[width=1\textwidth]{figures/supp_istd_mask.jpg}
    \caption{Examples of shadow masks in the ISTD+ dataset. Our mask is an intermediate soft shadow mask represented as a grayscale image, while all other masks are binary.}
    \label{istd_mask}
\end{figure*}

\begin{figure*}[t]
    \centering
    \includegraphics[width=1\textwidth]{figures/srd_sample_jpg.jpg}
    \caption{Illustrate the soft shadow image examples in the SRD dataset. The red boxes highlight the boundaries and regions of soft shadows, showcasing their blurry boundaries and gradual transitions in the penumbra area.}
    \label{srd_sample}
\end{figure*}

\begin{figure*}[t]
    \centering
    \includegraphics[width=0.99\textwidth]{figures/lrss_sample_jpg.jpg}
    \caption{Illustrate the soft shadow image examples in LRSS dataset.}
    \label{lrss_sample}
\end{figure*}

\begin{figure*}[t]
    \centering
    \includegraphics[width=0.99\textwidth]{figures/istd+_sample.png}
    \caption{Illustrate the hard shadow image examples in ISTD+ dataset.}
    \label{istd+_sample}
\end{figure*}

\begin{figure*}[t]
    \centering
    \includegraphics[width=0.99\textwidth]{figures/supp_visual_1.png}
    \caption{Examples of soft shadow image removal results on the SRD dataset~\cite{qu2017deshadownet}. The input shadow image, the estimated results of (a) BMNet~\cite{zhu2022bijective}, (b) ShadowDiffusion~\cite{guo2023shadowdiffusion}, Inpaint4Shadow~\cite{li2023leveraging}, (d) Homoformer~\cite{xiao2024homoformer}, and (e) Ours, as well as the ground truth image, respectively.}
    \label{SUPP}
\end{figure*}

\begin{figure*}[t]
    \centering
    \includegraphics[width=0.99\textwidth]{figures/supp_visual_2.png}
    \caption{Examples of shadow removal results on SRD datasets~\cite{qu2017deshadownet}. The input shadow image, the estimated results of (a) DC-ShadowNet~\cite{jin2021dc}, (b) DeS3~\cite{jin2024des3}, and (c) Ours, as well as the ground truth image, respectively.}
    \label{SUPP_2}
\end{figure*}
